# Supplementary material for: Analysis of DAWNBench, a Time-to-Accuracy Machine Learning Performance Benchmark
Source: arXiv:1806.01427 source file (2019-12-01)
Supplement: Supplementary file 1 [file appendix.tex]

\begin{appendix}

\begin{table}[t!]
\centering
\setlength\itemsep{2em}
\small
\begin{tabular}{ccc}
  \specialcell{Hardware}
    & \specialcell{\# of entries} \\ \hline
  GPU       & 8 \\
  TPU       & 0 \\
  CPU       & 0
\end{tabular}
\centering
\setlength\itemsep{2em}
\small
\begin{tabular}{ccc}
  \specialcell{Framework}
    & \specialcell{\# of entries} \\ \hline
  TensorFlow    & 2 \\
  PyTorch       & 6 \\
  Caffe         & 0 \\
  MXNet         & 0
\end{tabular}

\caption{Overview of hardware platform and software framework for
\dawnbench CIFAR10 submission.}
\vspace{-0.25em}
\label{table:cifar10-entry-stats}
\end{table}

%\section{CIFAR10 entries overview}
%We give an overview of the hardware and software platforms for CIFAR10 entries
%to \dawnbench in Table~\ref{table:cifar10-entry-stats}.
%
%
%
%\begin{figure}[t!]
%  \centering
%  \includegraphics[width=0.99\columnwidth]{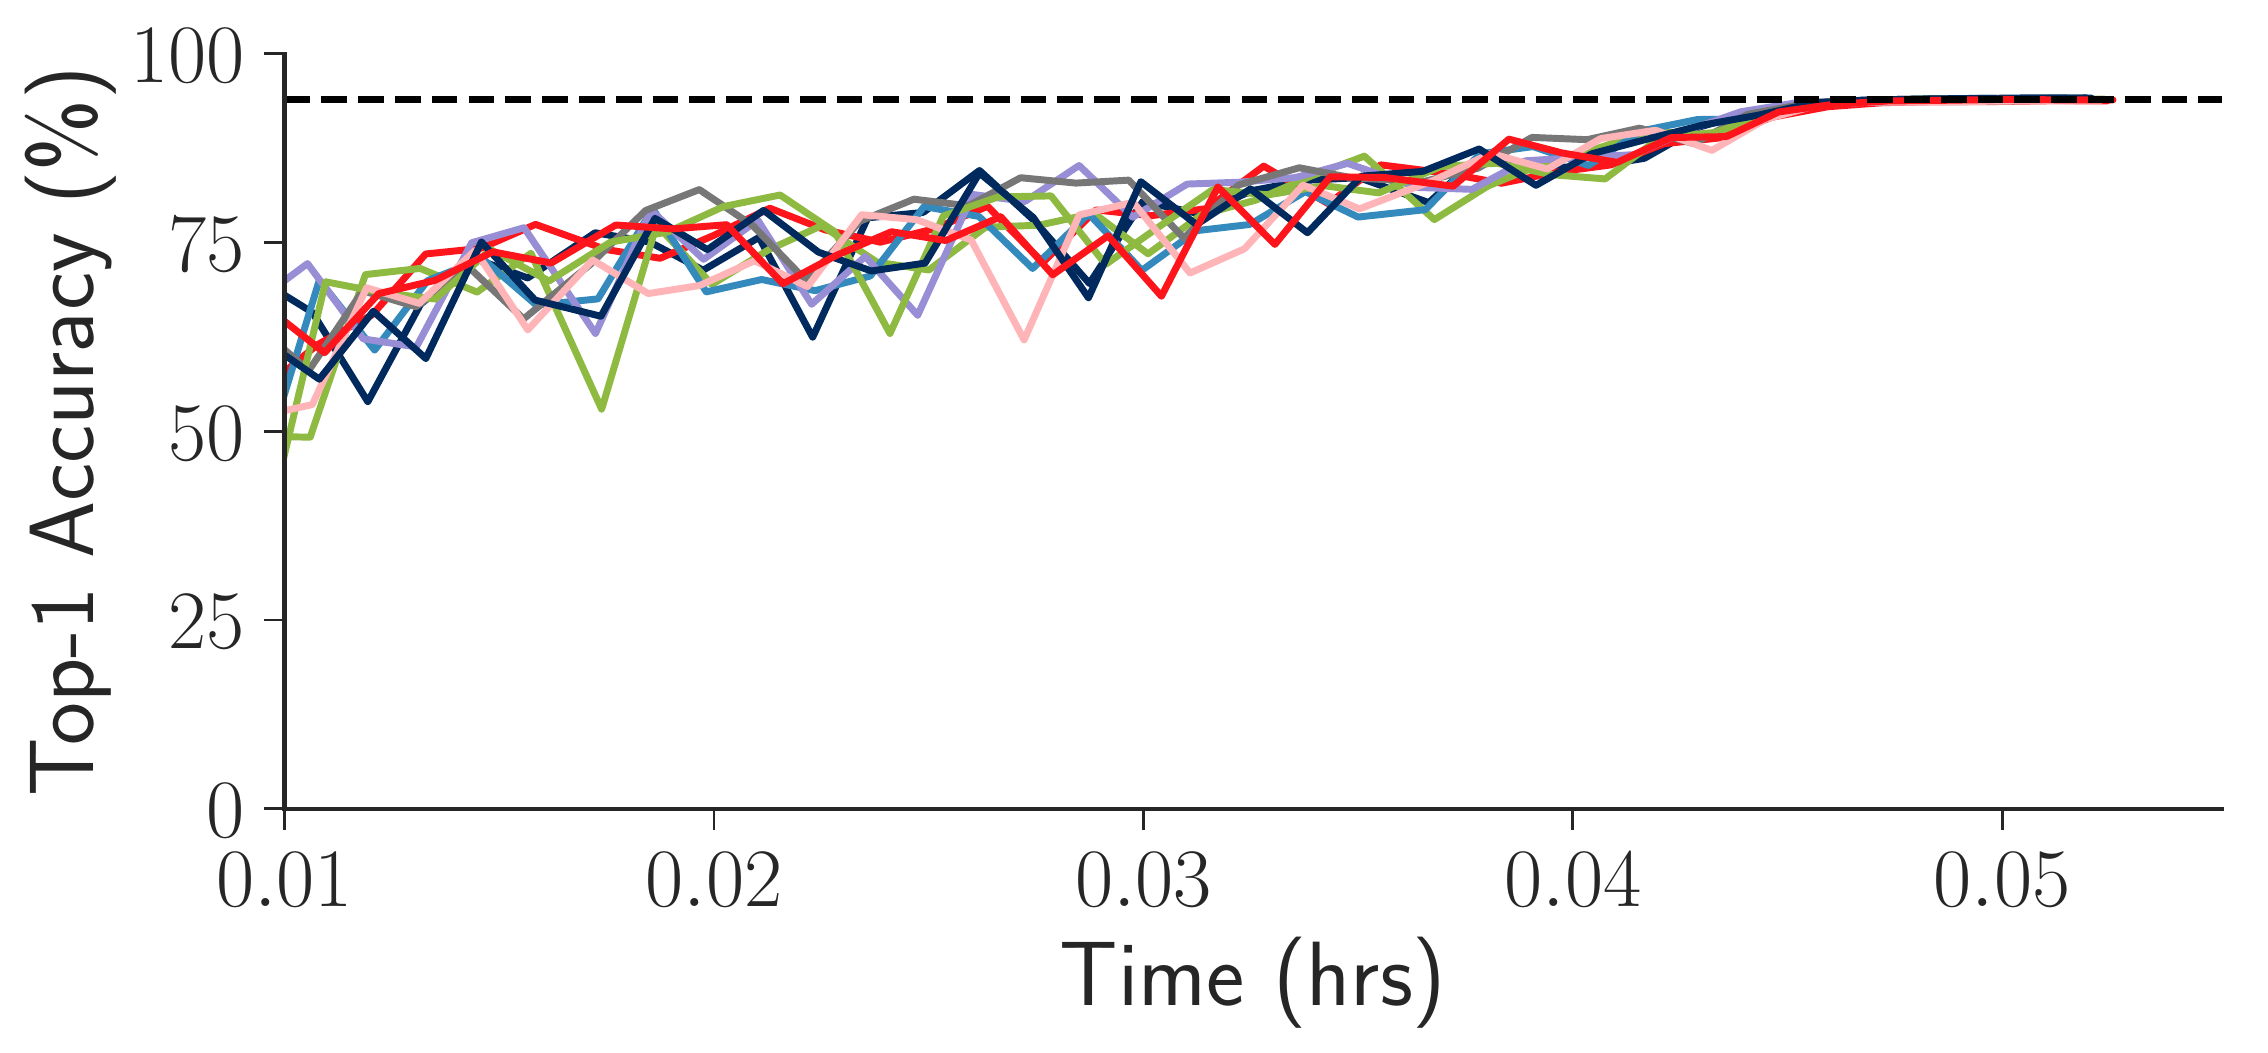}
%  \caption{
%      Validation accuracy over 10 training runs of fast.ai's custom Wide ResNet-34 (8 V100
%      GPUs) on CIFAR10 with an accuracy threshold of 94\% top-1 accuracy (dashed line).
%      Each trial is shown as a separate line.
%      The variance across runs is small near the accuracy thresholds.
%  }
%  \label{fig:stability-time-cifar10}
%  % \vspace{-1em}
%\end{figure}

\begin{table}[t!]
\centering
\setlength\itemsep{2em}
\small
\begin{tabular}{lccc}
  \specialcell{Entry name} & \specialcell{Coeff. of\\variation} & \specialcell{Frac. of runs} \\ \hline
  Wide ResNet-34, 8xV100   & 3.8\%                    & 50\% \\
  Wide ResNet-34, 1xV100   & 2.9\%                    & 70\% \\
  ResNet-18, 1xV100        & 1.4\%                    & 90\% \\
\end{tabular}
\caption{Coefficient of variation and fraction of runs that reached the desired target accuracy
  of the top single server blade entries for image classification on CIFAR10 (10 runs).}
\label{table:cifar10-entry-variance}
\end{table}

\input{tables/mlperf_official}

\input{tables/mlperf_aws}

%\section{Variance of Time-to-Accuracy}
%We show the variation for time-to-accuracy for CIFAR10 \dawnbench entries
%(Table~\ref{table:cifar10-entry-variance}), the official \mlperf entries
%(Table~\ref{table:mlperf-official-var-all}), and \mlperf entries reproduced in
%stable, public cloud (Table~\ref{table:mlperf-aws-var-all}).
%
%As shown, the coefficient of variation is less than 14\% for all entries except
%the distributed Transformer entries. However, \mlperf is planning to extended
%the dataset for Transformer, which we believe will reduce the coefficient of
%variation.
%
%\section{Entry Analysis for CIFAR-10}
%\begin{figure*}[t!]
%  \centering
%  \includegraphics[width=1.2\columnwidth]{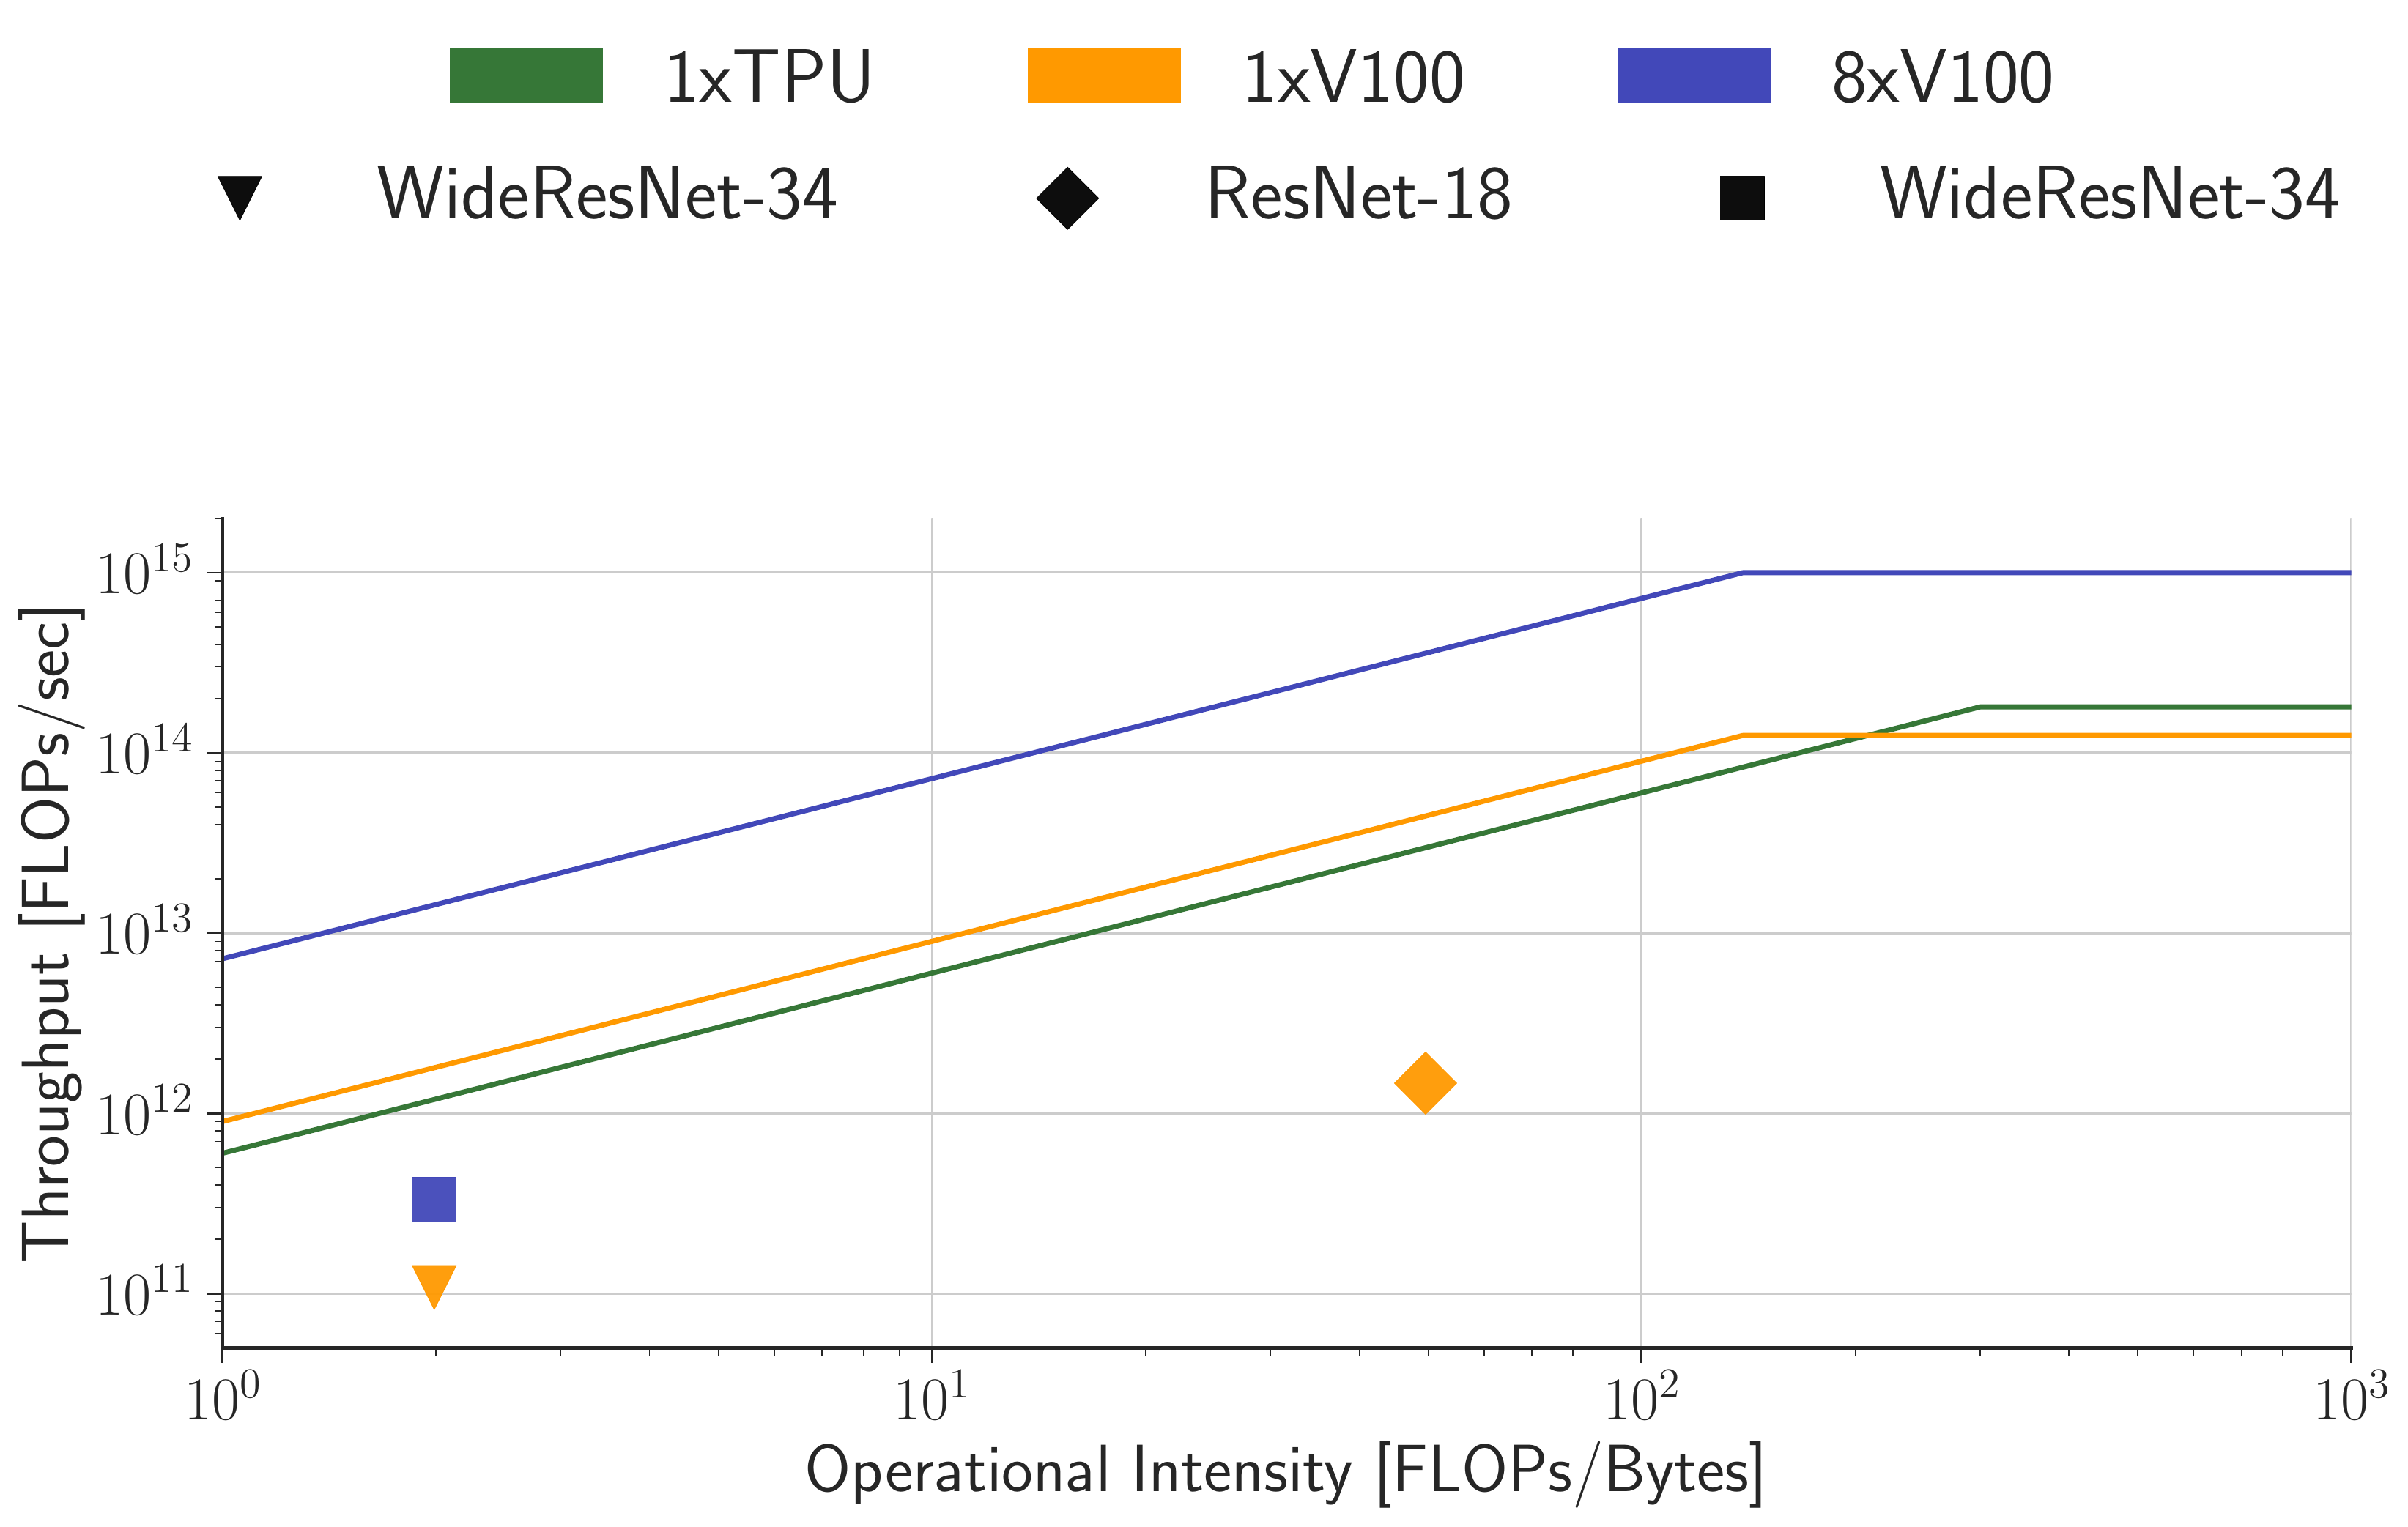}
%  \caption{
%    Roofline models for the various entries submitted to \dawnbench and \mlperf. All of the
%    entries under-utilize the hardware resources, by up to 10$\times$.
%  }
%  \label{fig:roofline}
%  \vspace{-0.5em}
%\end{figure*}

\end{appendix}
